# Supplementary material for: A Mountaineering Strategy to Excited States: Highly-Accurate Energies and Benchmarks for Exotic Molecules and Radicals
Source: arXiv:2003.04183 source file (2020-03-09)
Supplement: Supplementary file 1 [file Exotic-SI.pdf]

# A Mountaineering Strategy to Excited States: Highly-Accurate Energies and Benchmarks for Exotic Molecules and Radicals Supporting Information

Pierre-François Loos,[*,†] Anthony Scemama,[†] Martial Boggio-Pasqua,[†] and Denis Jacquemin[*,‡]

†*Laboratoire de Chimie et Physique Quantiques, Université de Toulouse, CNRS, UPS, France*

‡*Laboratoire CEISAM - UMR CNRS 6230, Université de Nantes, 2 Rue de la Houssinière, BP 92208, 44322 Nantes Cedex 3, France*

E-mail: loos@irsamc.ups-tlse.fr; Denis.Jacquemin@univ-nantes.fr

# S1 Basis set and frozen-core effects

Table S1: CC3 transition energies (in eV) determined with various basis sets. FC, SC, and full stand for frozen-core (large cores), small-core (freezing only the 1$s$ electrons) and correlating all electrons, respectively.

| | | 6-31+G(d) FC | *aug*-cc-pVDZ FC | *aug*-cc-pVTZ FC | *aug*-cc-pVQZ FC | *aug*-cc-pVQZ SC | *aug*-cc-pVQZ Full | *aug*-cc-pCVQZ Full | *aug*-cc-pV5Z FC |
|---|---|---|---|---|---|---|---|---|---|
| Carbonylfluoride | $^1A_2$ | 7.33 | 7.34 | 7.31 | 7.31 | | 7.29 | 7.28 | 7.31 |
| | $^3A_2$ | 7.03 | 7.05 | 7.03 | 7.03 | | 7.01 | 7.00 | 7.04 |
| $CCl_2$ | $^1B_1$ | 2.71 | 2.69 | 2.61 | 2.60 | 2.59 | 2.57 | 2.57 | 2.59 |
| | $^1A_2$ | 4.46 | 4.40 | 4.35 | 4.37 | 4.36 | 4.34 | 4.33 | 4.36 |
| | $^3B_1$ | 1.10 | 1.20 | 1.20 | 1.21 | 1.21 | 1.19 | 1.19 | 1.21 |
| | $^3A_2$ | 4.41 | 4.34 | 4.28 | 4.30 | 4.29 | 4.28 | 4.26 | 4.29 |
| CClF | $^1A''$ | 3.66 | 3.63 | 3.56 | 3.55 | 3.55 | 3.53 | 3.53 | 3.55 |
| $CF_2$ | $^1B_1$ | 5.18 | 5.12 | 5.07 | 5.06 | | 5.02 | 5.02 | 5.05 |
| | $^3B_1$ | 2.71 | 2.71 | 2.76 | 2.77 | | 2.75 | 2.75 | 2.77 |
| Difluorodiazirine | $^1B_1$ | 3.83 | 3.80 | 3.74 | 3.73 | | | | |
| | $^1A_2$ | 7.13 | 7.11 | 7.02 | 7.00 | | | | |
| | $^1B_2$ | 8.51 | 8.45 | 8.50 | 8.52 | | | | |
| | $^3B_1$ | 3.09 | 3.06 | 3.03 | 3.03 | | | | |
| | $^3B_2$ | 5.48 | 5.47 | 5.45 | 5.47 | | | | |
| | $^3B_1$ | 5.86 | 5.83 | 5.81 | 5.82 | | | | |
| Formylfluoride | $^1A''$ | 6.09 | 6.03 | 5.99 | 5.99 | | 5.98 | 5.97 | 6.00 |
| | $^3A''$ | 5.72 | 5.65 | 5.62 | 5.63 | | 5.62 | 5.61 | 5.64 |
| HCCl | $^1A''$ | 2.05 | 2.02 | 1.97 | 1.96 | 1.96 | 1.95 | 1.94 | 1.96 |
| HCF | $^1A''$ | 2.58 | 2.53 | 2.49 | 2.49 | | 2.47 | 2.47 | 2.49 |
| HCP | $^1\Sigma^-$ | 5.19 | 5.06 | 4.85 | 4.83 | 4.83 | 4.82 | 4.81 | 4.82 |
| | $^1\Delta$ | 5.48 | 5.33 | 5.15 | 5.12 | 5.11 | 5.11 | 5.09 | 5.10 |
| | $^3\Sigma^+$ | 3.44 | 3.47 | 3.45 | 3.46 | 3.46 | 3.46 | 3.44 | 3.47 |
| | $^3\Delta$ | 4.40 | 4.35 | 4.22 | 4.21 | 4.21 | 4.20 | 4.20 | 4.20 |
| HPO | $^1A''$ | 2.49 | 2.47 | 2.46 | 2.47 | 2.47 | 2.47 | 2.47 | 2.48 |
| HPS | $^1A''$ | 1.57 | 1.60 | 1.59 | 1.60 | 1.59 | 1.59 | 1.59 | 1.61 |
| HSiF | $^1A''$ | 3.09 | 3.08 | 3.07 | 3.07 | 3.06 | 3.06 | 3.06 | 3.07 |
| $SiCl_2$ | $^1B_1$ | 3.94 | 3.93 | 3.90 | 3.91 | 3.91 | 3.91 | 3.90 | 3.92 |
| | $^3B_1$ | 2.39 | 2.45 | 2.48 | 2.49 | 2.52 | 2.52 | 2.52 | 2.50 |
| Silylidene | $^1A_2$ | 2.14 | 2.18 | 2.15 | 2.16 | 2.15 | 2.16 | 2.15 | 2.16 |
| | $^1B_2$ | 3.88 | 3.81 | 3.78 | 3.79 | 3.78 | 3.78 | 3.78 | 3.80 |

# S2 Benchmark data

Table S2: Transition energies determined with various models for the exotic set. All values are in eV and have been obtained with the *aug*-cc-pVTZ basis set applying the FC approximation.

| | | TBE | CIS(D) | CC2 | EOM-MP2 | STEOM-CCSD | CCSD | CCSDR(3) | CCSDT-3 | CC3 | SOS-ADC(2) [TM] | SOS-CC2 [TM] | SCS-CC2 [TM] | SOS-ADC(2) [QM] | ADC(2) | ADC(3) | ADC(2.5) |
|---|---|---|---|---|---|---|---|---|---|---|---|---|---|---|---|---|---|
| Carbonylfluoride | $^1A_2$ | 7.31 | 7.38 | 7.47 | 7.39 | 7.07 | 7.36 | 7.32 | 7.32 | 7.31 | 7.27 | 7.48 | 7.47 | 7.04 | 7.22 | 7.32 | 7.27 |
| | $^3A_2$ | 7.06 | 7.08 | 7.14 | 7.08 | 6.82 | 7.03 | | | 7.03 | 7.05 | 7.24 | 7.21 | 6.81 | 6.91 | 7.01 | 6.96 |
| $CCl_2$ | $^1B_1$ | 2.59 | 2.59 | 2.58 | 2.36 | 2.35 | 2.61 | 2.59 | 2.61 | 2.61 | 2.58 | 2.67 | 2.64 | 2.44 | 2.46 | 2.41 | 2.44 |
| | $^1A_2$ | 4.40 | 4.20 | 4.27 | 4.27 | 4.33 | 4.57 | 4.37 | 4.41 | 4.35 | 4.50 | 4.61 | 4.50 | 4.29 | 4.12 | 4.76 | 4.44 |
| | $^3B_1$ | 1.22 | 1.09 | 1.15 | 0.84 | | 1.11 | | | 1.20 | 1.16 | 1.27 | 1.23 | 1.06 | 0.98 | 0.91 | 0.95 |
| | $^3A_2$ | 4.31 | 4.24 | 4.20 | 4.17 | 4.23 | 4.45 | | | 4.28 | 4.48 | 4.59 | 4.46 | 4.29 | 4.05 | 4.62 | 4.34 |
| CClF | $^1A''$ | 3.55 | 3.56 | 3.57 | 3.34 | 3.39 | 3.57 | 3.55 | 3.56 | 3.56 | 3.54 | 3.63 | 3.61 | 3.39 | 3.44 | 3.35 | 3.40 |
| $CF_2$ | $^1B_1$ | 5.09 | 5.06 | 5.09 | 4.90 | 4.90 | 5.09 | 5.07 | 5.08 | 5.07 | 5.05 | 5.15 | 5.13 | 4.89 | 4.94 | 4.86 | 4.90 |
| | $^3B_1$ | 2.77 | 2.63 | 2.70 | 2.47 | 2.61 | 2.69 | | | 2.76 | 2.74 | 2.84 | 2.79 | 2.64 | 2.54 | 2.48 | 2.51 |
| Difluorodiazirine | $^1B_1$ | 3.74 | 3.89 | 3.74 | 3.94 | 3.56 | 3.83 | 3.76 | 3.75 | 3.74 | 3.97 | 3.97 | 3.90 | 3.77 | 3.74 | 3.52 | 3.63 |
| | $^1A_2$ | 7.00 | 7.46 | 7.19 | 7.24 | | 7.10 | 7.05 | 7.02 | 7.02 | 7.29 | 7.28 | 7.25 | 7.10 | 7.19 | 6.70 | 6.95 |
| | $^1B_2$ | 8.52 | 8.53 | 8.29 | 8.90 | | 8.69 | 8.55 | 8.55 | 8.50 | 8.95 | 8.82 | 8.65 | 8.77 | 8.42 | 8.50 | 8.46 |
| | $^3B_1$ | 3.03 | 3.17 | 3.03 | 3.17 | 2.91 | 3.07 | | | 3.03 | 3.32 | 3.33 | 3.23 | 3.14 | 3.01 | 2.77 | 2.89 |
| | $^3B_2$ | 5.44 | 5.89 | 5.77 | 5.97 | | 5.40 | | | 5.45 | 5.53 | 5.55 | 5.63 | 5.41 | 5.72 | 5.04 | 5.38 |
| | $^3B_1$ | 5.80 | 6.13 | 5.99 | 5.71 | 5.59 | 5.84 | | | 5.81 | 6.20 | 6.21 | 6.13 | 6.05 | 5.97 | 5.47 | 5.72 |
| Formylfluoride | $^1A''$ | 5.96 | 6.03 | 6.14 | 6.00 | 5.88 | 6.02 | 5.99 | 6.00 | 5.99 | 5.99 | 6.19 | 6.17 | 5.78 | 5.91 | 5.93 | 5.92 |
| | $^3A''$ | 5.73 | 5.63 | 5.70 | 5.60 | 5.51 | 5.60 | | | 5.62 | 5.67 | 5.85 | 5.80 | 5.48 | 5.50 | 5.54 | 5.52 |
| HCCl | $^1A''$ | 1.98 | 1.95 | 1.91 | 1.65 | 1.80 | 1.99 | 1.95 | 1.98 | 1.97 | 2.01 | 2.06 | 2.01 | 1.88 | 1.84 | 1.81 | 1.83 |
| HCF | $^1A''$ | 2.49 | 2.54 | 2.44 | 2.19 | 2.32 | 2.51 | 2.48 | 2.50 | 2.49 | 2.51 | 2.58 | 2.53 | 2.38 | 2.34 | 2.30 | 2.32 |
| HCP | $^1\Sigma^-$ | 4.84 | 5.07 | 5.07 | 4.83 | 4.90 | 4.87 | 4.85 | 4.84 | 4.85 | 5.02 | 5.07 | 5.07 | 4.91 | 5.02 | 4.37 | 4.70 |
| | $^1\Delta$ | 5.15 | 5.40 | 5.41 | 5.12 | 5.22 | 5.16 | 5.16 | 5.14 | 5.15 | 5.23 | 5.29 | 5.33 | 5.12 | 5.33 | 4.66 | 5.00 |
| | $^3\Sigma^+$ | 3.47 | 3.74 | 3.73 | 3.55 | 3.41 | 3.36 | | | 3.45 | 3.37 | 3.38 | 3.50 | 3.30 | 3.69 | 3.10 | 3.40 |
| | $^3\Delta$ | 4.22 | 4.44 | 4.43 | 4.23 | 4.20 | 4.17 | | | 4.22 | 4.47 | 4.52 | 4.49 | 4.39 | 4.39 | 3.79 | 4.09 |
| HPO | $^1A''$ | 2.47 | 2.54 | 2.50 | 2.44 | 2.45 | 2.54 | 2.48 | 2.48 | 2.46 | 2.57 | 2.68 | 2.62 | 2.39 | 2.35 | 2.35 | 2.35 |
| HPS | $^1A''$ | 1.59 | 1.68 | 1.68 | 1.39 | 1.55 | 1.67 | 1.59 | 1.60 | 1.59 | 1.74 | 1.79 | 1.75 | 1.60 | 1.62 | 1.39 | 1.51 |
| HSiF | $^1A''$ | 3.05 | 3.16 | 3.14 | 2.78 | 3.02 | 3.12 | 3.07 | 3.08 | 3.07 | 3.22 | 3.24 | 3.21 | 3.12 | 3.11 | 2.88 | 3.00 |
| $SiCl_2$ | $^1B_1$ | 3.91 | 3.99 | 3.99 | 3.70 | 3.80 | 3.96 | 3.89 | 3.91 | 3.90 | 4.01 | 4.04 | 4.02 | 3.89 | 3.95 | 3.76 | 3.86 |
| | $^3B_1$ | 2.48 | 2.40 | 2.39 | 2.18 | | 2.45 | | | 2.48 | 2.51 | 2.52 | 2.48 | 2.44 | 2.35 | 2.31 | 2.33 |
| Silylidene | $^1A_2$ | 2.11 | 2.39 | 2.37 | 2.09 | 2.21 | 2.29 | 2.16 | 2.17 | 2.15 | 2.35 | 2.35 | 2.35 | 2.24 | 2.37 | 1.87 | 2.12 |
| | $^1B_2$ | 3.78 | 3.91 | 3.85 | 3.66 | 3.81 | 3.88 | 3.79 | 3.80 | 3.78 | 3.98 | 3.94 | 3.91 | 3.87 | 3.88 | 3.40 | 3.64 |

Table S3: Transition energies determined with various models for the radical set. All values are in eV and have been obtained with the *aug*-cc-pVTZ basis set applying the FC approximation.

| | | TBE | U-CCSD | RO-CCSD | U-CC3 | RO-CC3 |
|---|---|---|---|---|---|---|
| Allyl | $^2B_1$ | 3.39 | 3.70 | 3.48 | 3.48 | 3.44 |
| | $^2A_1$ | 4.99 | 5.12 | 5.01 | 4.97 | 4.95 |
| BeF | $^2\Pi$ | 4.14 | 4.18 | 4.18 | 4.15 | 4.15 |
| | $^2\Sigma^+$ | 6.21 | 6.31 | 6.31 | 6.21 | 6.21 |
| BeH | $^2\Pi$ | 2.49 | 2.51 | 2.51 | 2.50 | 2.50 |
| | $^2\Pi$ | 6.46 | 6.47 | 6.47 | 6.46 | 6.46 |
| $BH_2$ | $^2B_1$ | 1.18 | 1.20 | 1.20 | 1.19 | 1.20 |
| CH | $^2\Delta$ | 2.91 | 3.18 | 3.17 | 3.11 | 3.10 |
| | $^2\Sigma^-$ | 3.29 | 4.58 | 4.39 | 3.61 | 3.55 |
| | $^2\Sigma^+$ | 3.98 | 5.47 | 5.36 | 4.45 | 4.40 |
| $CH_3$ | $^2A_1'$ | 5.85 | 5.89 | 5.87 | 5.86 | 5.85 |
| | $^2E'$ | 6.96 | 7.00 | 6.98 | 6.97 | 6.97 |
| | $^2E'$ | 7.18 | 7.21 | 7.20 | 7.19 | 7.19 |
| | $^2A_2''$ | 7.65 | 7.67 | 7.66 | 7.65 | 7.65 |
| CN | $^2\Pi$ | 1.34 | 1.56 | 1.34 | 1.40 | 1.36 |
| | $^2\Sigma^+$ | 3.22 | 3.54 | 3.35 | 3.31 | 3.26 |
| CNO | $^2\Sigma^+$ | 1.61 | 2.24 | 2.25 | 1.75 | 1.77 |
| | $^2\Pi$ | 5.49 | 5.68 | 5.60 | 5.52 | 5.51 |
| $CO^+$ | $^2\Pi$ | 3.28 | 3.60 | 3.29 | 3.33 | 3.29 |
| | $^2\Sigma^+$ | 5.81 | 6.21 | 6.02 | 5.76 | 5.68 |
| $F_2BO$ | $^2B_1$ | 0.73 | 0.74 | 0.73 | 0.71 | 0.71 |
| | $^2A_1$ | 2.80 | 2.84 | 2.83 | 2.79 | 2.79 |
| $F_2BS$ | $^2B_1$ | 0.51 | 0.51 | 0.49 | 0.48 | 0.48 |
| | $^2A_1$ | 2.99 | 3.03 | 3.01 | 2.94 | 2.93 |
| $H_2BO$ | $^2B_1$ | 2.15 | 2.14 | 2.13 | 2.17 | 2.17 |
| | $^2A_1$ | 3.49 | 3.53 | 3.51 | 3.52 | 3.52 |
| HCO | $^2A''$ | 2.09 | 2.14 | 2.13 | 2.10 | 2.11 |
| | $^2A'$ | 5.45 | 5.54 | 5.53 | 5.44 | 5.44 |
| HOC | $^2A''$ | 0.92 | 0.95 | 0.93 | 0.93 | 0.93 |
| $H_2PO$ | $^2A''$ | 2.80 | 2.91 | 2.91 | 2.83 | 2.83 |
| | $^2A'$ | 4.21 | 4.26 | 4.27 | 4.21 | 4.23 |
| $H_2PS$ | $^2A''$ | 1.16 | 1.18 | 1.14 | 1.16 | 1.15 |
| | $^2A'$ | 2.72 | 2.79 | 2.77 | 2.75 | 2.75 |
| NCO | $^2\Sigma^+$ | 2.89 | 3.04 | 2.94 | 2.94 | 2.86 |
| | $^2\Pi$ | 4.73 | 5.01 | 5.02 | 4.80 | 4.81 |
| $NH_2$ | $^2A_1$ | 2.12 | 2.13 | 2.12 | 2.13 | 2.12 |
| Nitromethyl | $^2B_2$ | 2.05 | 2.47 | 2.46 | 2.06 | 2.05 |
| | $^2A_2$ | 2.38 | 2.71 | 2.71 | 2.47 | 2.46 |
| | $^2A_1$ | 2.56 | 2.94 | 2.93 | 2.56 | 2.55 |
| | $^2B_1$ | 5.35 | 5.59 | 5.56 | 5.38 | 5.36 |
| NO | $^2\Sigma^+$ | 6.13 | 6.23 | 6.21 | 6.13 | 6.12 |
| | $^2\Sigma^+$ | 7.29 | 7.40 | 7.38 | 7.30 | 7.28 |
| OH | $^2\Sigma^+$ | 4.10 | 4.14 | 4.13 | 4.13 | 4.13 |
| | $^2\Sigma^-$ | 8.02 | 7.75 | 7.76 | 7.66 | 7.66 |
| $PH_2$ | $^2A_1$ | 2.77 | 2.81 | 2.78 | 2.78 | 2.77 |
| Vinyl | $^2A''$ | 3.26 | 3.51 | 3.35 | 3.34 | 3.30 |
| | $^2A''$ | 4.69 | 4.91 | 4.80 | 4.76 | 4.73 |
| | $^2A'$ | 6.20 | 6.38 | 6.32 | 6.22 | 6.24 |

# S3 Multi-reference approaches for CON

Table S4: Vertical transition energies (eV) of CON. All calculations using a full valence active space of (15e,12o) and the *aug*-cc-pVTZ basis set. NEVPT2 calculations are performed within the partially-contracted scheme whereas CASPT2 calculations use a level shift of 0.3 a.u. and a IPEA of 0.25 a.u.

| State | Active space $(a_1, b_1, b_2, a_2)$ | State-average $(A_1, B_1, B_2, A2)$ | CASSCF | NEVPT2 | CASPT2 | MRCI |
|---|---|---|---|---|---|---|
| $^4\Pi(\pi \rightarrow \pi^\star)$ | (6,3,3,0) | (0,2,2,0) | 3.01 | 2.72 | 2.74 | 2.81 |
| $^2\Pi(\pi \rightarrow \pi^\star)$ | (6,3,3,0) | (0,2,2,0) | 3.94 | 3.52 | 3.55 | 3.62 |
| $^2\Sigma^+(n \rightarrow \pi^\star)$ | (6,3,3,0) | (1,1,1,0) | 3.85 | 3.81 | 3.72 | 3.83 |
| $^2\Phi(\pi \rightarrow \pi^\star)$ | (6,3,3,0) | (0,2,2,0) | 4.86 | 4.32 | 4.35 | 4.44 |

# S4 Geometries

## S4.1 Exotic compounds

Below, we provide the Cartesian coordinates of the exotic compounds investigated in this study. These are given in atomic units (bohr) and they have been obtained at the CC3(full)/*aug*-cc-pVTZ level of theory.

### S4.1.1 Carbonylfluoride ($F_2CO$)

```
C     0.00000000          0.00000000         -0.30652633
O     0.00000000          0.00000000         -2.52469534
F     0.00000000          2.00254958          1.16003038
F     0.00000000         -2.00254958          1.16003038
```

### S4.1.2 $CCl_2$

```
C     0.00000000          0.00000000         -1.60920674
Cl    0.00000000          2.65360612          0.27602958
Cl    0.00000000         -2.65360612          0.27602958
```

### S4.1.3 CClF

```
C     0.29776085          0.00000000          1.47969075
F     2.16980264          0.00000000         -0.10569879
Cl   -2.46756349          0.00000000         -0.32822320
```

### S4.1.4 $CF_2$

```
C     0.00000000          0.00000000         -1.14170749
F     0.00000000          1.94810617          0.36114458
F     0.00000000         -1.94810617          0.36114458
```

### S4.1.5 Difluorodiazirine ($CF_2N_2$)

| | | | |
|---|---|---|---|
| C | 0.00000000 | 0.00000000 | -0.15283028 |
| F | 0.00000000 | 2.06077297 | -1.57706828 |
| F | 0.00000000 | -2.06077297 | -1.57706828 |
| N | 1.20382241 | 0.00000000 | 2.20566821 |
| N | -1.20382241 | 0.00000000 | 2.20566821 |

### S4.1.6 Formylfluoride (FHCO)

| | | | |
|---|---|---|---|
| C | 0.00536098 | 0.00000000 | 0.75320959 |
| O | 2.17369813 | 0.00000000 | 0.22287752 |
| H | -0.83846350 | 0.00000000 | 2.62640974 |
| F | -1.84051320 | 0.00000000 | -0.99373750 |

### S4.1.7 HCCl

| | | | |
|---|---|---|---|
| H | -1.88068369 | 0.00000000 | -0.14323924 |
| Cl | 2.28559426 | 0.00000000 | -0.43261163 |
| C | -0.40491057 | 0.00000000 | 1.32161964 |

### S4.1.8 HCF

| | | | |
|---|---|---|---|
| C | -0.13561085 | 0.00000000 | 1.20394474 |
| F | 1.85493976 | 0.00000000 | -0.27610752 |
| H | -1.71932891 | 0.00000000 | -0.18206846 |

### S4.1.9 HCP

| | | | |
|---|---|---|---|
| H | 0.00000000 | 0.00000000 | -4.03090449 |
| C | 0.00000000 | 0.00000000 | -2.01691641 |
| P | 0.00000000 | 0.00000000 | 0.91401621 |

### S4.1.10 HPO

| | | | |
|---|---|---|---|
| H | 0.31668637 | 0.00000000 | 0.14072725 |
| P | -0.80573521 | 0.00000000 | 2.65136926 |
| O | 1.43391190 | 0.00000000 | 4.38886277 |

### S4.1.11 HPS

| | | | |
|---|---|---|---|
| H | -2.56278959 | 0.00000000 | 2.36296006 |
| P | 0.09114182 | 0.00000000 | 1.82568543 |
| S | 0.07946992 | 0.00000000 | -1.85778170 |

### S4.1.12 HSiF

| | | | |
|---|---|---|---|
| Si | -0.06438136 | 0.00000000 | 1.67253150 |
| F | 2.24990164 | 0.00000000 | -0.33928119 |
| H | -2.18552027 | 0.00000000 | -0.28748154 |

### S4.1.13 $SiCl_2$

| | | | |
|---|---|---|---|
| Si | 0.00000000 | 0.00000000 | -1.78528322 |
| Cl | 0.00000000 | 3.04414528 | 0.71619419 |
| Cl | 0.00000000 | -3.04414528 | 0.71619419 |

### S4.1.14 Silylidene ($H_2CSi$)

| | | | |
|---|---|---|---|
| C | 0.00000000 | 0.00000000 | -2.09539928 |
| Si | 0.00000000 | 0.00000000 | 1.14992930 |
| H | 0.00000000 | 1.70929524 | -3.22894481 |
| H | 0.00000000 | -1.70929524 | -3.22894481 |

## S4.2 Radicals

Below, we provide the Cartesian coordinates of the radical compounds investigated in this study. These are given in atomic units (bohr) and they have been obtained at the UCCSD(T)(full)/*aug*-cc-pVTZ level of theory, except when noted.

### S4.2.1 Allyl ($C_3H_5$)

| | | | |
|---|---|---|---|
| C | 0.00000000 | 0.00000000 | 0.83050732 |
| C | 0.00000000 | 2.30981224 | -0.38722841 |
| C | 0.00000000 | -2.30981224 | -0.38722841 |
| H | 0.00000000 | 0.00000000 | 2.87547067 |
| H | 0.00000000 | 4.06036949 | 0.65560561 |
| H | 0.00000000 | -4.06036949 | 0.65560561 |
| H | 0.00000000 | 2.41059890 | -2.42703281 |
| H | 0.00000000 | -2.41059890 | -2.42703281 |

### S4.2.2 BeF

| | | | |
|---|---|---|---|
| Be | 0.00000000 | 0.00000000 | -1.77936990 |
| F | 0.00000000 | 0.00000000 | 0.79083149 |

### S4.2.3 BeH

| | | | |
|---|---|---|---|
| Be | 0.00000000 | 0.00000000 | 0.25103976 |
| H | 0.00000000 | 0.00000000 | -2.24485003 |

### S4.2.4 $BH_2$

| | | | |
|---|---|---|---|
| B | 0.00000000 | 0.00000000 | 0.14984923 |
| H | 0.00000000 | 2.01119016 | -0.81846345 |
| H | 0.00000000 | -2.01119016 | -0.81846345 |

### S4.2.5 CH

| | | | |
|---|---|---|---|
| C | 0.00000000 | 0.00000000 | -0.16245872 |
| H | 0.00000000 | 0.00000000 | 1.93436816 |

### S4.2.6 $CH_3$

| | | | |
|---|---|---|---|
| C | 0.00000000 | 0.00000000 | 0.00000000 |
| H | 0.00000000 | 0.00000000 | 2.03379507 |
| H | 0.00000000 | 1.76131924 | -1.01689753 |
| H | 0.00000000 | -1.76131924 | -1.01689753 |

### S4.2.7 CN

| | | | |
|---|---|---|---|
| C | 0.00000000 | 0.00000000 | -1.18953886 |
| N | 0.00000000 | 0.00000000 | 1.01938091 |

### S4.2.8 CNO

| | | | |
|---|---|---|---|
| C | 0.00000000 | 0.00000000 | -2.50680714 |
| N | 0.00000000 | 0.00000000 | -0.22402176 |
| O | 0.00000000 | 0.00000000 | 2.07682752 |

### S4.2.9 CON

Optimized at the U-CCSDT/cc-pVTZ level.

| | | | |
|---|---|---|---|
| C | 0.00000000 | 0.00000000 | -2.44062558 |
| O | 0.00000000 | 0.00000000 | -0.20455596 |
| N | 0.00000000 | 0.00000000 | 2.32515818 |

### S4.2.10 $CO^+$

| | | | |
|---|---|---|---|
| C | 0.00000000 | 0.00000000 | -1.20324172 |
| O | 0.00000000 | 0.00000000 | 0.90271821 |

### S4.2.11 $F_2BO$

| | | | |
|---|---|---|---|
| O | 0.00000000 | 0.00000000 | 2.65260017 |
| B | 0.00000000 | 0.00000000 | 0.07681654 |
| F | 0.00000000 | 2.16433924 | -1.13888019 |
| F | 0.00000000 | -2.16433924 | -1.13888019 |

### S4.2.12 $F_2BS$

| | | | |
|---|---|---|---|
| S | 0.00000000 | 0.00000000 | 2.64960984 |
| B | 0.00000000 | 0.00000000 | -0.74406239 |
| F | 0.00000000 | 2.14169276 | -2.01390354 |
| F | 0.00000000 | -2.14169276 | -2.01390354 |

### S4.2.13 $H_2BO$

| | | | |
|---|---|---|---|
| O | 0.00000000 | 0.00000000 | 1.17360276 |
| B | 0.00000000 | 0.00000000 | -1.27133435 |
| H | 0.00000000 | 1.98370787 | -2.36904602 |
| H | 0.00000000 | -1.98370787 | -2.36904602 |

### S4.2.14 HCO

| | | | |
|---|---|---|---|
| H | 0.00000000 | -2.55038496 | 1.39798104 |
| C | 0.00000000 | -1.17300976 | -0.19046167 |
| O | 0.00000000 | 1.04073447 | 0.05480615 |

### S4.2.15 HOC

| | | | |
|---|---|---|---|
| H | 0.00000000 | 1.82002973 | 1.50851586 |
| O | 0.00000000 | 0.96467865 | -0.12887834 |
| C | 0.00000000 | -1.43868535 | 0.04508983 |

### S4.2.16 $H_2PO$

| | | | |
|---|---|---|---|
| P | 0.00000000 | 0.87766783 | -0.10010856 |
| O | 0.00000000 | -1.95912323 | 0.05701315 |
| H | 2.08101554 | 2.05955113 | 1.08591181 |
| H | -2.08101554 | 2.05955113 | 1.08591181 |

### S4.2.17 $H_2PS$

| | | | |
|---|---|---|---|
| P | 0.00000000 | 1.81994516 | -0.10769248 |
| S | 0.00000000 | -1.93707861 | 0.02086846 |
| H | 2.03762554 | 2.75934101 | 1.32385757 |
| H | -2.03762554 | 2.75934101 | 1.32385757 |

### S4.2.18 NCO

| | | | |
|---|---|---|---|
| N | 0.00000000 | 0.00000000 | -2.39343558 |
| C | 0.00000000 | 0.00000000 | -0.07238136 |
| O | 0.00000000 | 0.00000000 | 2.14968523 |

### S4.2.19 $NH_2$

| | | | |
|---|---|---|---|
| N | 0.00000000 | 0.00000000 | 0.15111603 |
| H | 0.00000000 | 1.51574744 | -1.04982949 |
| H | 0.00000000 | -1.51574744 | -1.04982949 |

### S4.2.20 Nitromethyl ($CH_2$-$NO_2$)

| | | | |
|---|---|---|---|
| C | 0.00000000 | 0.00000000 | -2.58417104 |
| N | 0.00000000 | 0.00000000 | 0.08692471 |
| O | 0.00000000 | -2.06715629 | 1.15098225 |
| O | 0.00000000 | 2.06715629 | 1.15098225 |
| H | 0.00000000 | 1.81656349 | -3.48616378 |
| H | 0.00000000 | -1.81656349 | -3.48616378 |

### S4.2.21 NO

| | | | |
|---|---|---|---|
| N | 0.00000000 | 0.00000000 | -1.15775086 |
| O | 0.00000000 | 0.00000000 | 1.01357658 |

### S4.2.22 OH

| | | | |
|---|---|---|---|
| O | 0.00000000 | 0.00000000 | -0.10864763 |
| H | 0.00000000 | 0.00000000 | 1.72431679 |

### S4.2.23 $PH_2$

| | | | |
|---|---|---|---|
| P | 0.00000000 | 0.00000000 | 0.11427641 |
| H | 0.00000000 | 1.91899987 | -1.75604411 |
| H | 0.00000000 | -1.91899987 | -1.75604411 |

### S4.2.24 Vinyl ($C_2H_3$)

| | | | |
|---|---|---|---|
| C | 0.00000000 | 1.16769663 | -0.04303146 |
| C | 0.00000000 | -1.29945364 | 0.15810072 |
| H | 0.00000000 | 2.38429609 | 1.59801822 |
| H | 0.00000000 | 2.08759130 | -1.87998309 |
| H | 0.00000000 | -2.90307925 | -1.08814513 |
